# Supplementary material for: Characterizing Out-of-Distribution Error via Optimal Transport
Source: arXiv:2305.15640 source file (2023-10-27)
Supplement: Supplementary file 1 [file supp.tex]

\documentclass{article}

% if you need to pass options to natbib, use, e.g.:
%     \PassOptionsToPackage{numbers, compress}{natbib}
% before loading neurips_2023

% ready for submission
\usepackage{neurips_2023}

% to compile a preprint version, e.g., for submission to arXiv, add add the
% [preprint] option:
%     \usepackage[preprint]{neurips_2023}

% to compile a camera-ready version, add the [final] option, e.g.:
%     \usepackage[final]{neurips_2023}

% to avoid loading the natbib package, add option nonatbib:
%    \usepackage[nonatbib]{neurips_2023}

\usepackage{tabularx,booktabs}
\usepackage[utf8]{inputenc} % allow utf-8 input
\usepackage[T1]{fontenc}    % use 8-bit T1 fonts
\usepackage{hyperref}       % hyperlinks
\usepackage{url}            % simple URL typesetting
\usepackage{booktabs}       % professional-quality tables
\usepackage{amsfonts}       % blackboard math symbols
\usepackage{nicefrac}       % compact symbols for 1/2, etc.
\usepackage{microtype}      % microtypography
\usepackage{xcolor}         % colors
\usepackage[utf8]{inputenc} % allow utf-8 input
\usepackage[T1]{fontenc}    % use 8-bit T1 fonts
\usepackage{hyperref}       % hyperlinks
\usepackage{url}            % simple URL typesetting
\usepackage{booktabs}       % professional-quality tables
\usepackage{amsfonts}       % blackboard math symbols
\usepackage{nicefrac}       % compact symbols for 1/2, etc.
\usepackage{microtype}      % microtypography
\usepackage{adjustbox}
\usepackage{multirow}
\usepackage{subcaption}

%%% HELPER CODE FOR DEALING WITH EXTERNAL REFERENCES
\usepackage{xr}
\makeatletter
\newcommand*{\addFileDependency}[1]{
  \typeout{(#1)}
  \@addtofilelist{#1}
  \IfFileExists{#1}{}{\typeout{No file #1.}}
}
\makeatother
\newcommand*{\myexternaldocument}[1]{
    \externaldocument{#1}
    \addFileDependency{#1.tex}
    \addFileDependency{#1.aux}
}
%%% END HELPER CODE

% put all the external documents here!
\myexternaldocument{NeurIPS 2023/neurips_2023}

% \usepackage{zref-xr}
% \makeatletter
% \zexternaldocument[A-]{main}
% \AtBeginDocument{%
%   \setcounter{equation}{\zref@extractdefault{A-eq-last}{default}{0}}%
%   \zref@refused{A-eq-last}%
%   \setcounter{thm}{\zref@extractdefault{A-thm-last}{default}{0}}%
%   \zref@refused{A-thm-last}%
% }
% \makeatother

\usepackage{amsmath,amssymb,amsthm,bbm}

\title{Characterizing Out-of-Distribution Error \\ via Optimal Transport (Appendix)}

% The \author macro works with any number of authors. There are two commands
% used to separate the names and addresses of multiple authors: \And and \AND.
%
% Using \And between authors leaves it to LaTeX to determine where to break the
% lines. Using \AND forces a line break at that point. So, if LaTeX puts 3 of 4
% authors names on the first line, and the last on the second line, try using
% \AND instead of \And before the third author name.

\author{Yuzhe Lu$^*$$^1$, Yilong Qin$^*$$^1$, Andrew Shen$^1$, Ketong Chen$^{1}$, Zhenlin Wang$^{1}$, Runtian Zhai$^{1}$ \\
\textbf{Soheil Kolouri$^2$, Joseph Campbell$^1$,  Simon Stepputtis$^1$, Katia Sycara$^{1}$} \\
$^1$Carnegie Mellon University \ \ $^2$Vanderbilt University \\ 
{\small \texttt{\{yuzhelu, yilongq, andrews, ketongc, zhenlinw, rzhai, sstepput, jcampbell, sycara\}@cs.cmu.edu} } \\ 
{\small \texttt{soheil.kolouri@vanderbilt.edu}}
}

\begin{document}

\maketitle

\appendix
\input{NeurIPS 2023/supplementary}
\bibliographystyle{plain}
\bibliography{reference}

%%%%%%%%%%%%%%%%%%%%%%%%%%%%%%%%%%%%%%%%%%%%%%%%%%%%%%%%%%%%

\end{document}
